# Supplementary material for: Secure Data Sharing With Flow Model
Source: arXiv:2009.11762 source file (2020-09-24)
Supplement: Supplementary file 1 [file appendix.tex]

\appendix
\section{Additional proofs}

In this improved solution, we need to assume that the data provider has a secret labeling function $g$ that can compute the ground truth labels for the input data. For example, this labeling function can be human experts who have domain knowledge and are willing to provide labels.

%We consider the image classification problem as an example: Let $\mathcal{D}$ be a distribution of images, and each sample in the domain of $\mathcal{D}$ has a label, where there are finite kinds of labels in total. We have $n$ samples of $\mathcal{D}$ and the labeling function of the images, and want another person to train a classifier using these data. This case is common in some areas where labeling the data are much more expensive than collecting unlabeled data. For instance, for medical images, labeling requires much expert knowledge in this field but collecting unlabeled images is much easier.

For this problem, we use Algorithm \ref{alg:enc} to design a new algorithm:

\begin{algorithm}[htbp]
   \caption{Private Image Classification}
   \label{alg:class}
\begin{algorithmic}
   \STATE {\bfseries Input:} original images $\{s_i\}_{i=1}^n$, labeling function $g$
   \STATE Sample $A_1, A_2$ uniformly from all orthogonal matrices
   \STATE Run Algorithm \ref{alg:enc} with $A_1$ and get $Enc_1(s_i)$
   \STATE Run Algorithm \ref{alg:enc} with $A_2$ and get $Enc_2(s_i)$
   \FOR{$i=1$ {\bfseries to} $n$}
   \STATE $y_i=g(Enc_2(s_i))$
   \ENDFOR
   \STATE {\bfseries Output:} $\{(Enc_1(s_i), y_i)\}_{i=1}^n$
\end{algorithmic}
\end{algorithm}

This algorithm ensures that the labeling function is safe even if matrix $A_1$ is leaked to the adversary:
\begin{theorem}
\label{extension-thm}
The success probability of any strong adversary trying to recover $A_2$ with tolerance $\theta$ cannot exceed $\delta(\mathcal{H}_0^n, \mathcal{H}_1^n)+\theta$.
\end{theorem}
The proof of Theorem \ref{extension-thm} is very similar to Theorem \ref{main-thm}, so we only provide a proof sketch here: Note that $A_2$ is totally independent of $A_1$, so knowing $A_1$ doesn't influence the encryption by $A_2$. We can assume that the adversary successfully solved the encryption of the images and only work on the labels, which falls into the proof framework of Theorem \ref{main-thm}.

% \textbf{\emph{Do not put content after the references.}}
% %
% Put anything that you might normally include after the references in a separate
% supplementary file.

% We recommend that you build supplementary material in a separate document.
% If you must create one PDF and cut it up, please be careful to use a tool that
% doesn't alter the margins, and that doesn't aggressively rewrite the PDF file.
% pdftk usually works fine. 

% \textbf{Please do not use Apple's preview to cut off supplementary material.} In
% previous years it has altered margins, and created headaches at the camera-ready
% stage. 
